# Supplementary material for: Can MLLMs Reason in Multimodality? EMMA: An Enhanced MultiModal ReAsoning Benchmark
Source: arXiv:2501.05444 source file (2025-01-09)
Supplement: Supplementary file 1 [file supp.tex]

%auto-ignore
\documentclass[10pt,twocolumn,letterpaper]{article}

%%%%%%%%% PAPER TYPE  - PLEASE UPDATE FOR FINAL VERSION
% \usepackage{cvpr}              % To produce the CAMERA-READY version
\usepackage[review]{cvpr}      % To produce the REVIEW version
% \usepackage[pagenumbers]{cvpr} % To force page numbers, e.g. for an arXiv version

% Import additional packages in the preamble file, before hyperref
\input{preamble}
% Include other packages here, before hyperref.
% \usepackage{subfigure}
\usepackage{graphicx}
\graphicspath{{assets/}} %Setting the graphicspath
\usepackage{amsmath}
\usepackage{amssymb}
\usepackage{booktabs}
\usepackage{enumitem}
\usepackage{algorithm}
\usepackage{algpseudocode}
\usepackage{bm}
\usepackage{multirow}
\usepackage{caption}
\usepackage{subcaption}
\usepackage{tikz}
\usepackage{tabularx}

\usepackage{pifont}% http://ctan.org/pkg/pifont

\usepackage{lipsum}
\usepackage{bbm}
\usepackage{dsfont}
\usepackage{makecell}

% It is strongly recommended to use hyperref, especially for the review version.
% hyperref with option pagebackref eases the reviewers' job.
% Please disable hyperref *only* if you encounter grave issues, e.g. with the
% file validation for the camera-ready version.
%
% If you comment hyperref and then uncomment it, you should delete
% ReviewTempalte.aux before re-running LaTeX.
% (Or just hit 'q' on the first LaTeX run, let it finish, and you
%  should be clear).
% \usepackage[pagebackref,breaklinks,colorlinks]{hyperref}

\makeatletter
\makeatother

% It is strongly recommended to use hyperref, especially for the review version.
% hyperref with option pagebackref eases the reviewers' job.
% Please disable hyperref *only* if you encounter grave issues, 
% e.g. with the file validation for the camera-ready version.
%
% If you comment hyperref and then uncomment it, you should delete *.aux before re-running LaTeX.
% (Or just hit 'q' on the first LaTeX run, let it finish, and you should be clear).
\definecolor{cvprblue}{rgb}{0.21,0.49,0.74}
\usepackage[pagebackref,breaklinks,colorlinks,citecolor=cvprblue]{hyperref}

% Support for easy cross-referencing
\usepackage[capitalize]{cleveref}
\crefname{section}{Sec.}{Secs.}
\Crefname{section}{Section}{Sections}
\Crefname{table}{Table}{Tables}
\crefname{table}{Tab.}{Tabs.}

%\newcommand{\jw}[1]{\textbf{\textcolor{blue}{#1}}}

%%%%%%%%% PAPER ID  - PLEASE UPDATE
 % *** Enter the Paper ID here

\begin{document}
% \clearpage
% \setcounter{page}{1}
% \maketitlesupplementary
\appendix
\title{Can MLLMs Reason in Multimodality? EMMA: An Enhanced MultiModal ReAsoning Benchmark\\Supplementary Materials}
\maketitle
\input{supp_text}

\clearpage
{\small
\bibliographystyle{ieee_fullname}
\bibliography{egbib}
}
\end{document}
